# Supplementary material for: Observation of Pines' Demon in Sr$_2$RuO$_4$
Source: arXiv:2007.06670 source file (2022-05-27)
Supplement: Supplementary file 1 [file Husain-SRO-Demon-Preprint-v9-supplement.pdf]

## I. SUPPLEMENTARY METHODS

### A. Sample Growth and Characterization

Millimeter-sized, high-quality single crystals of $Sr_2RuO_4$ for M-EELS and STEM-EELS experiments were grown by a floating-zone technique reported previously [1]. Crystals were verified to have a superconducting transition temperature of about 1.5 K by AC susceptibility. Samples for M-EELS were cleaved in UHV to reveal atomically flat surfaces. A focused ion beam (FIB) lamella oriented along the ab-plane was prepared for STEM-EELS using an FEI Scios 2 FIB instrument.

### B. M-EELS Measurements

Momentum-resolved Electron Energy-Loss Spectroscopy (M-EELS) measurements were carried out with an HR-EELS spectrometer modified for both high momentum accuracy and precision [2] (see Fig. S5). The primary beam energy was chosen to be 50 eV, with energy and momentum resolutions of 6 meV and 0.03 $\text{Å}^{-1}$, respectively.

Single crystals of $Sr_2RuO_4$ were mounted onto oxygen-free high-conductivity copper pucks (Fig. S1a) along with an aluminum top post using silver epoxy (EPOTEK H20-E) cured at 120 C. Samples were cleaved at 300 K in $\sim 1.5 \times 10^{-10}$ torr vacuum and were oriented *in situ* based on the (0,0) and (1,0) Bragg reflections as observed with M-EELS at zero energy loss (Fig. S1b). Only cleaves resulting in atomically flat surfaces and resolution-limited Bragg reflections were used for the measurements reported here. The out-of-plane momentum transfer was held fixed at $q = 3.95$ $\text{Å}^{-1}$ (i.e., $L = 8$) throughout the entire experiment.

M-EELS spectra of the high-energy continuum were obtained by dividing out the momentum-dependent Coulomb matrix element and antisymmetrizing to remove the Bose factor [2]. It is noteworthy that, under certain conditions, neglecting the effects of the Coulomb matrix element can result in an artificially dispersing loss peak with dispersion velocity equal to the velocity of the incident probe electron ( 27.6 eV $\cdot$ Å for a 50 eV electron). This artifact arises due to the combination of geometry and the Coulomb matrix element and only occurs when the magnitude of the probe electron's momentum perpendicular to the surface is larger after scattering (i.e. backward scattering) [3]. We avoid this geomet-

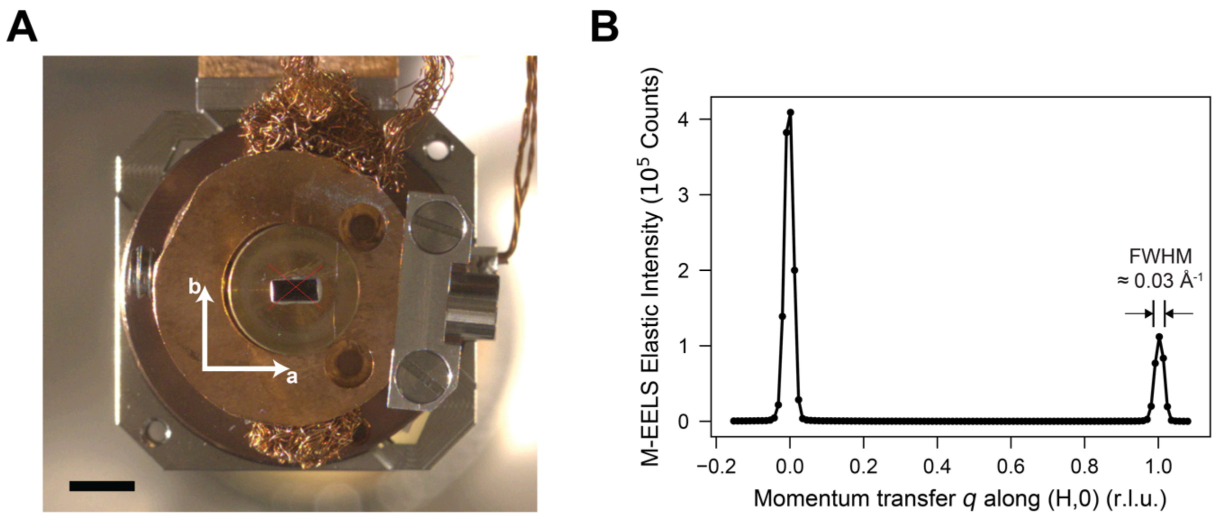


FIG. S1. Cleaved $Sr_2RuO_4$ single crystal measured with M-EELS. (A) Example $Sr_2RuO_4$ single crystal measured with M-EELS. The sample is mounted on an OFHC copper puck and cleaved in UHV to reveal a flat surface (scale bar 5 mm). To accurately align the instrument momentum transfer with the crystal axes, the sample is rotated azimuthally via a piezorotator. In this case the a-axis was aligned to be in the scattering plane. (B) Momentum-dependence of the elastic M-EELS response, which corresponds to Bragg diffraction, of $Sr_2RuO_4$ along $(H, 0)$. A sharp specular peak at $(0, 0)$ is visible, as is a $(1, 0)$ LEED reflection with a FWHM of approximately 0.03 $\text{Å}^{-1}$, indicating a clean, well ordered surface.

ric artifact by both dividing out the Coulomb matrix element and always working in the forward-scattering geometry where the magnitude of the outgoing momentum perpendicular to the surface is smaller after scattering [2]. In any case, one should note that such geometric effects are irrelevant in the low-energy demon regime because the probe electron velocity at 50 eV is around fifty times larger than that of the demon.

M-EELS spectra of the high-energy continuum, shown in Fig. 3 of the main manuscript, were scaled for visibility. The spectra at different momenta were multiplied by a factor of $q^2$ and scaled so that their energy-integrated first moment is equal to that of the optical charge susceptibility in the same energy region (i.e. scaled to $-\frac{\pi}{2m}N_{eff}$, where $N_{eff} = 3.21 \times 10^{-4}$ $\text{Å}^{-3}$ and $m$ is the free electron mass) [4]. This scaling effectively gives the spectra units of $\text{eV}^{-1}\text{Å}^{-3}$.

### C. STEM-EELS Measurements

The high-energy continuum shown in Fig. 3 of the main manuscript closely resembles that observed previously in $Bi_2Sr_2CaCu_2O_{8+x}$ [5, 6], suggesting it may be a generic high-energy property of strange metals. To test whether this continuum is a property of the bulk, we performed transmission EELS measurements on the same materials.

Scanning transmission electron microscopy EELS (STEM-EELS) measurements were performed within a Nion UltraSTEM instrument at Rutgers University with a 60 keV primary beam energy and a full-width-at-half-maximum energy resolution of 10 meV. The angular convergence semi-angle of the beam was 30 mrad. Combined with the size of the exit aperture, these experiments probe a momentum range centered at $q = 0$ with a width $\Delta q = 5.94$ $\text{Å}^{-1} \simeq 3.5$ r.l.u., so can be considered a fully momentum-integrated measurement. STEM-EELS was performed on a single-crystal lamella of $Sr_2RuO_4$ oriented with the ab-plane perpendicular to the incident electron beam. This lamella was lifted out and thinned down to electron transparency using an FEI Scios 2 Focused Ion Beam instrument.

STEM-EELS spectra were acquired in a crystalline region approximately 45 nm thick ($t/\lambda \sim 0.8$ with $\lambda \simeq 60$ nm at 60 keV) and integrated over the non-energy-dispersive direction of a 2D CMOS gain-corrected image with an acceptance semi-angle of 16 mrad. From there, the momentum-integrated dynamic charge susceptibility, $\chi''(\omega)$, was obtained by antisymmetrizing to remove the Bose factor and then applying the same normalization as was done for M-EELS (see Section I.B above).

A comparison between M-EELS and STEM-EELS data from $Sr_2RuO_4$ is shown in Fig. S2. The spectra from the two techniques are nearly identical. While the STEM-EELS data are momentum-integrated, this comparison is meaningful because the continuum observed in M-EELS measurements is momentum-independent (main manuscript Fig. 3). This comparison therefore verifies the bulk nature of the high-energy continuum in $Sr_2RuO_4$ .

### D. Surface Passivation

Proper surface preparation is critical for reliable M-EELS measurements of $Sr_2RuO_4$ . When cleaved in ultrahigh vacuum at cryogenic temperatures, the surface of $Sr_2RuO_4$ forms dangling bonds that result in a partially filled band and a surface state whose origin is

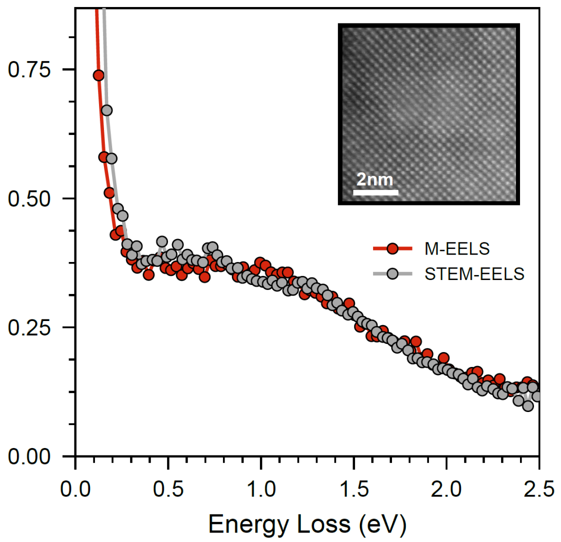


FIG. S2. Comparison between surface M-EELS and bulk-sensitive EELS measurements of $Sr_2RuO_4$ with a scanning transmission electron microscope (STEM). The similarity of the two spectra verifies the bulk origin of the high-energy continuum. (Inset) high-angle annular dark field image of the sample region used for STEM-EELS measurements confirms its crystallinity.

unrelated to the bulk electronic structure [7, 8]. This surface state complicated interpretation of early ARPES experiments [9, 10], and could result in an extraneous 2D surface state plasmon in M-EELS measurements of the sort observed on some transition metal surfaces [11, 12] . The cleaved surface of $Sr_2RuO_4$ also exhibits a $\sqrt{2}\times\sqrt{2}$ lattice reconstruction associated with coordinated rotation of the $RuO_6$ octahedra [13]. This superstructure results in band folding that is clearly visible in ARPES experiments [8]. Obtaining bulk-like properties in surface experiments requires suppressing both the surface state and the lattice reconstruction [8].

In Ref. [7], Stoger et al. demonstrated that CO exposure passivates the surface state of $Sr_2RuO_4$ by forming metal carboxylate groups that terminate the dangling surface bonds [7]. This reaction has an activation barrier of 0.17 eV, so complete passivization of the surface takes a few hours at cryogenic temperatures [7, 8] and is essentially instantaneous at room temperature. CO passivization also disorders the $\sqrt{2} \times \sqrt{2}$ reconstruction, suppressing the surface band folding, resulting in pristine bulk bands in ARPES that match both electronic structure calculations and the observed periods in quantum oscillation experiments [1, 8, 14].

We therefore cleaved our surfaces at room temperature, rather than at cryogenic temperature, and then exposed them for several hours to residual CO gas with a partial pressure of $3 \times 10^{-11}$ torr—a net exposure of order $\sim 0.25$ Langmuir. At this exposure, the surface should be fully passivated. We confirmed that this procedure results in a disordered $\sqrt{2} \times \sqrt{2}$ reconstruction by measuring the (1/2,1/2) surface LEED reflection and confirming that it is weak and highly broadened with a width $\Delta H \sim 0.2$ r.l.u. [15]. In all other respects, the surface is crystallographically perfect, as demonstrated by the resolution-limited specular and (1,0) LEED reflections shown in Fig. S1. M-EELS measurements on these surfaces should therefore be reliable and exhibit properties representative of the bulk, as demonstrated in Ref. [8].

### E. Anisotropy of the High-Energy Continuum

The band structure of $Sr_2RuO_4$ is anisotropic in the $(a, b)$ plane, as is the dispersion of the Demon mode shown in Fig. 4 of the main manuscript. It is therefore important to characterize whether the high-energy continuum (main manuscript Fig 3) is similarly anisotropic. We measured the continuum at a single momentum $q = 0.5$ r.l.u. along the $(1, 1)$ direction, i.e., $(H, K) = (\frac{\sqrt{2}}{2}, \frac{\sqrt{2}}{2})$, to compare with $q = 0.5$ r.l.u. along $(1, 0)$. These spectra are shown in Fig. S3. We find that the response is very similar along the two directions, suggesting that the strange metal fluctuations are isotropic in-plane, despite the strong anisotropy of other aspects of the electronic structure.

### F. Temperature Dependence of the High-Energy Continuum

The high-energy continuum in $Sr_2RuO_4$ is slightly temperature dependent. As shown in Fig. S4, when the temperature is reduced from 300 K to 30 K, the continuum is slightly reduced at lower energy. This behavior mimics that observed previously in overdoped $Bi_2Sr_2CaCu_2O_{8+x}$ [5], and is consistent with the widely held belief that, while $Sr_2RuO_4$ has some strange metal properties at high temperature and high energy scales, at low temperature it is more Fermi liquid like.

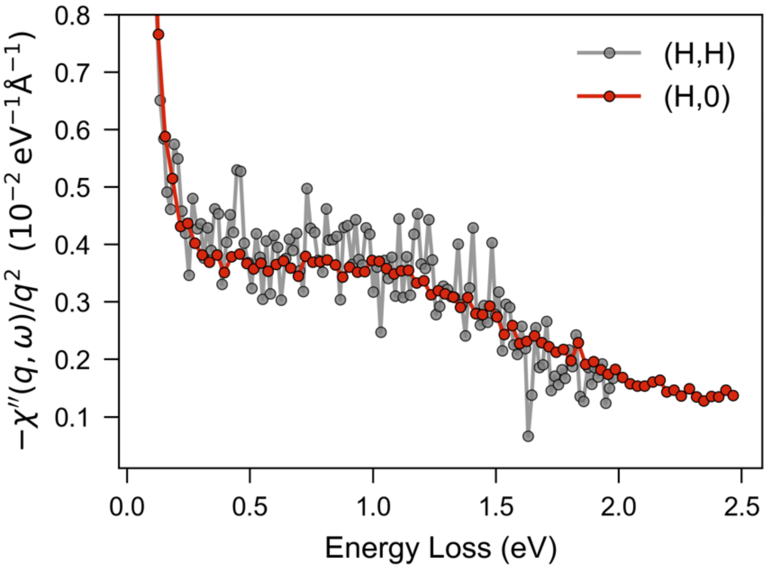


FIG. S3. **Isotropic high-energy continuum in $Sr_2RuO_4$ .** Comparison of the M-EELS response at $q = 0.5$ r.l.u. along the $(H, 0)$ and $(H, H)$ directions. To within the statistical uncertainty of the data, the overall shape of the strange metal continuum is the same in both directions. This observation suggests that the high-energy, continuum is roughly anisotropic in $Sr_2RuO_4$ .

### G. Momentum resolution of HR-EELS vs. M-EELS

Previous HR-EELS studies of $Sr_2RuO_4$ did not observe the demon mode [13] (main manuscript Fig. 4. The reason is differences in the momentum resolution of HR-EELS compared to M-EELS. The demon is rapidly dispersing, and is only visible at momenta $q < q_c = 0.08$ r.l.u.. As illustrated in Fig. S5, the momentum resolution in Ref. [13], measured by the FWHM of the specular reflection, is $0.14\text{Å}^{-1} \sim 0.08$ r.l.u.. This measurement therefore integrated over the entire dispersion curve of the demon. By comparison, the same measurement for our M-EELS instrument yields a resolution of 0.017 r.l.u. (Fig. S5). This improved $q$ resolution allows the demon to be visible.

### H. Fitting the Demon Mode

The dispersions of the acoustic Demon mode and the 67 meV optical phonon shown in Fig. 4 of the main text were determined by fitting the quasi-elastic line to a pseudo-

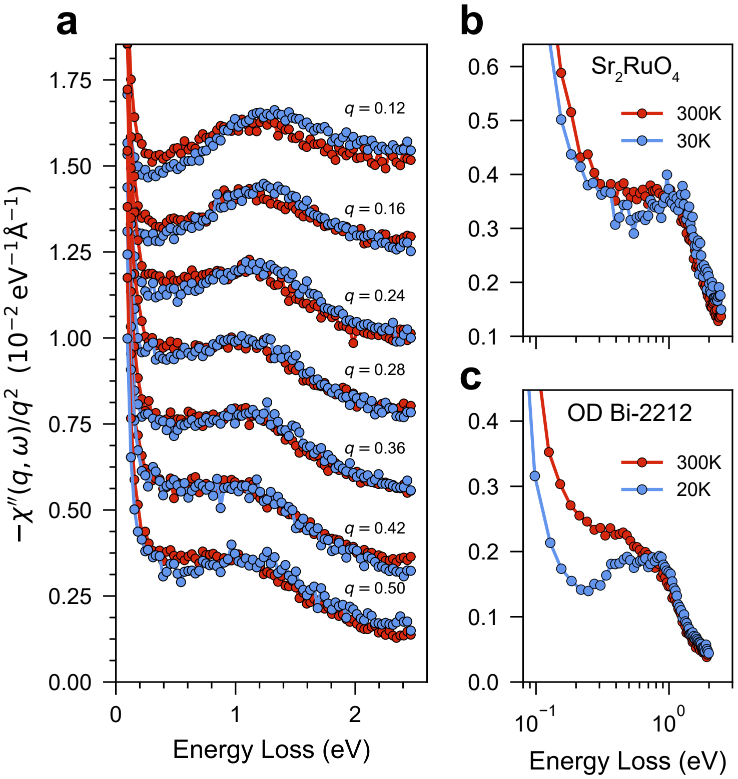


FIG. S4. **Temperature dependence of the high energy continuum in $\mathbf{Sr_2RuO_4}$ .** The spectral weight at low energy is slightly reduced at low temperature, exhibiting the same behavior as overdoped $Bi_2Sr_2CaCu_2O_{8+x}$ [5, 6].

Voigt function (i.e., a weighted sum of a Gaussian and Lorentzian), the acoustic mode to a an antisymmetrized Lorentzian, the 67 meV optical phonon to a Fano profile (following previous work in refs [13, 16], and the 25 meV, 35 meV, and 50 meV optical phonons (when present) to Lorentzians. For these fits we focused on the raw data, i.e., before dividing the matrix elements or antisymmetrizing. The error bars in Fig. 3 represent the confidence interval determined from the chi-squared value and the corresponding diagonal component of the covariance matrix from fits of this model to the experimental data. Sample fits are shown in Fig. S6. Line plots of the demon dispersion, i.e., of the data from Fig. 4 in the main manuscript, are shown in Fig. S7.

As the dispersion of optical phonons is well-documented experimentally and theoretically [13, 16], we focus here on the acoustic demon mode. The FWHM of the mode is plotted

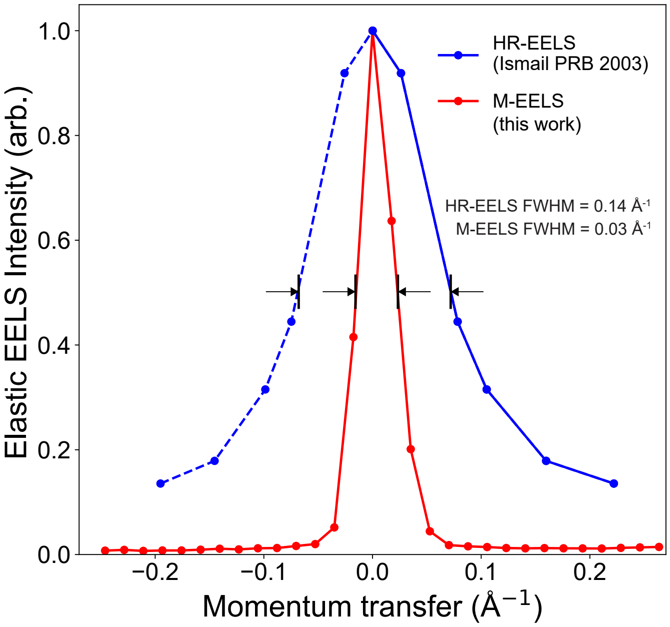


FIG. S5. **Comparison of the momentum resolution of HR-EELS vs. M-EELS**. Plot of the elastic specular reflection from the surface of $Sr_2RuO_4$ as a function of momentum transfer for HR-EELS from ref. [13] (blue), and for M-EELS from this work (red). The HR-EELS data were mirrored (dashed line) to obtain the FWHM since Ref. [13] presented only positive values of $q$. The full-width at half-maximum of the specular reflection for M-EELS is about 0.03 Å$^{-1}$, which is nearly five times sharper than that of HR-EELS (0.14 Å$^{-1}$), despite working at a significantly higher beam energy (50 eV compared to 20 eV). Because the demon only exists below about 0.13 Å$^{-1}$ or 0.08 r.l.u., it was not visible in HR-EELS measurements.

in Fig. S8, which shows that the linewidth grows with increasing momentum. Some of this width is due to the steep dispersion of the mode and the finite momentum resolution of the M-EELS measurement. However, the linewidth becomes nearly 40 meV by $q \sim 0.07$ r.l.u., indicating that intrinsic decay channels are also present. The increasing width with $q$ is most likely a consequence of Landau damping, which is commonly observed in conventional plasmons in metals [17]. For momenta $q > 0.08$ r.l.u., the mode is overdamped and no longer visible, identifying $q_c = 0.08$ r.l.u. as its critical momentum.

At lower temperature, $T = 30$ K, there is a slight sharpening of the demon mode. This may be due to the reduction in the single-particle continuum shown in Fig. S4, which could

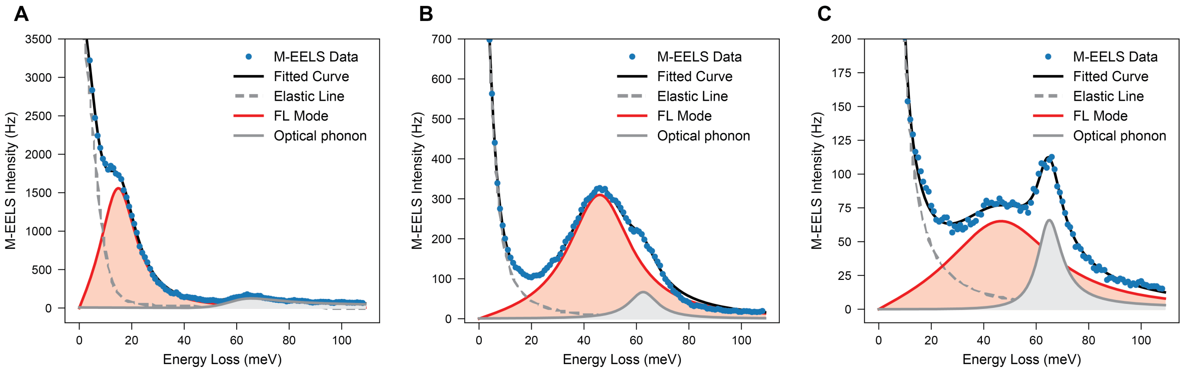


FIG. S6. **Example fits of the phonon and demon modes**. Three example fits of the M-EELS spectra for (A) q=0.03 r.l.u. along $(1,1)$ at 300 K, (B) q=0.06 r.l.u. along $(1,0)$ at 300 K, and (C) q=0.08 r.l.u. along $(1,0)$ at 30 K. Fits comprise a quasi-elastic line (grey dashed line) of pseudo-Voigt form, a demon mode using a Lorentz oscillator (red), and optical phonons (grey full lines) each with a Fano lineshape.

result in fewer decay channels.

For $q \leq 0.02$ r.l.u., the Demon mode is no longer resolvable from the tail of the quasi-elastic line due to the finite energy and momentum resolution of the experiment (Fig. S9). The mode energy is therefore indistinguishable from zero and can be considered gapless. In this momentum region, the vertical error bars in Fig. 3 of the main manuscript represent bounds. The value of this bound is subject to systematic errors that depend on the model used. To make an estimate of this bound, we fix the elastic line to be a Gaussian and attribute the non-Gaussian tail to the Demon mode through two different schemes. In scheme A, we attribute all of this extra tail to the demon mode. In scheme B, we attribute the non-Gaussian tail to a sum of the demon and an unresolvable "scheme B mode." We then place the upper bound on the peak position in energy of the demon mode in Fig. 3 at the larger of the two values. At $q = 0.00$ $\text{\AA}^{-1}$ (Fig. S9) the upper bound on the demon energy gap is 8 meV.

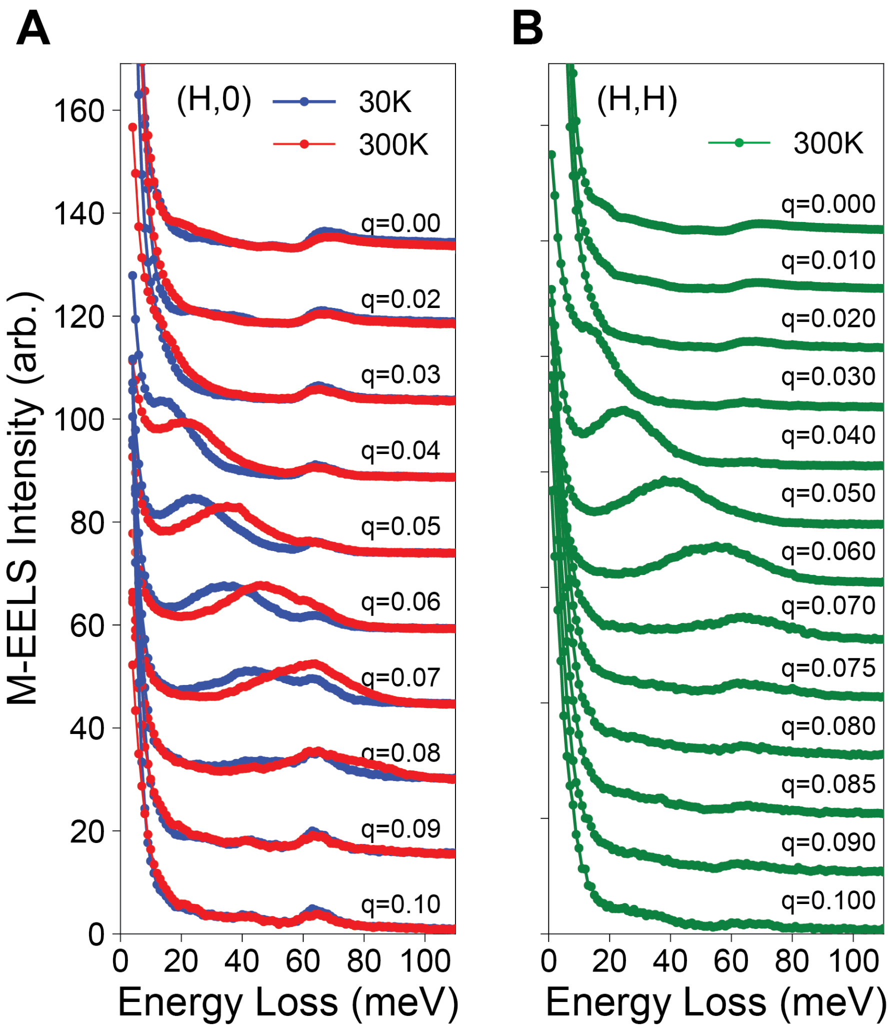


FIG. S7. **Line plots of the dispersion of the demon mode**. Line plots of the M-EELS spectra from Fig. 4 of them main manuscript, showing the dispersion of the demon mode along (A) $(1, 0)$ at 30 K (blue), 300 K (red) and (B) along $(1, 1)$ at 300 K (green). Spectra are offset vertically and normalized to their values at 85 meV for clarity.

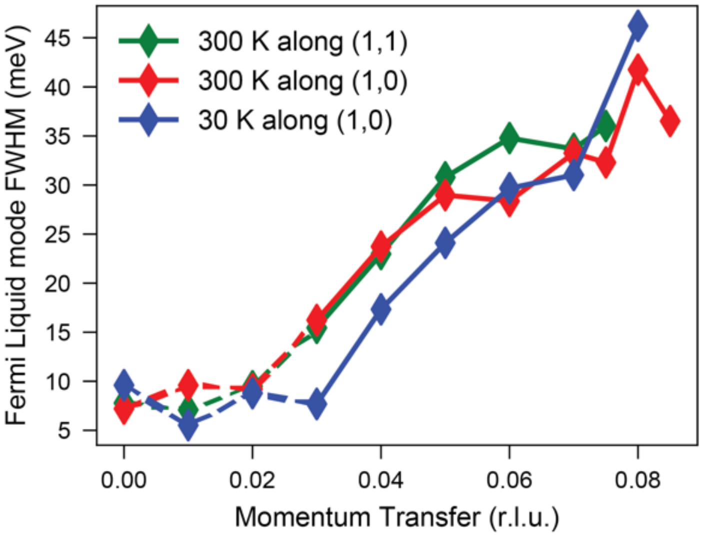


FIG. S8. **Width of the demon mode**. Full-width at half-maximum energy width of the demon mode as a function of momentum, $q$. The width ranges from around 8 meV at 0.03 r.l.u. to over 40 meV at 0.08 r.l.u.

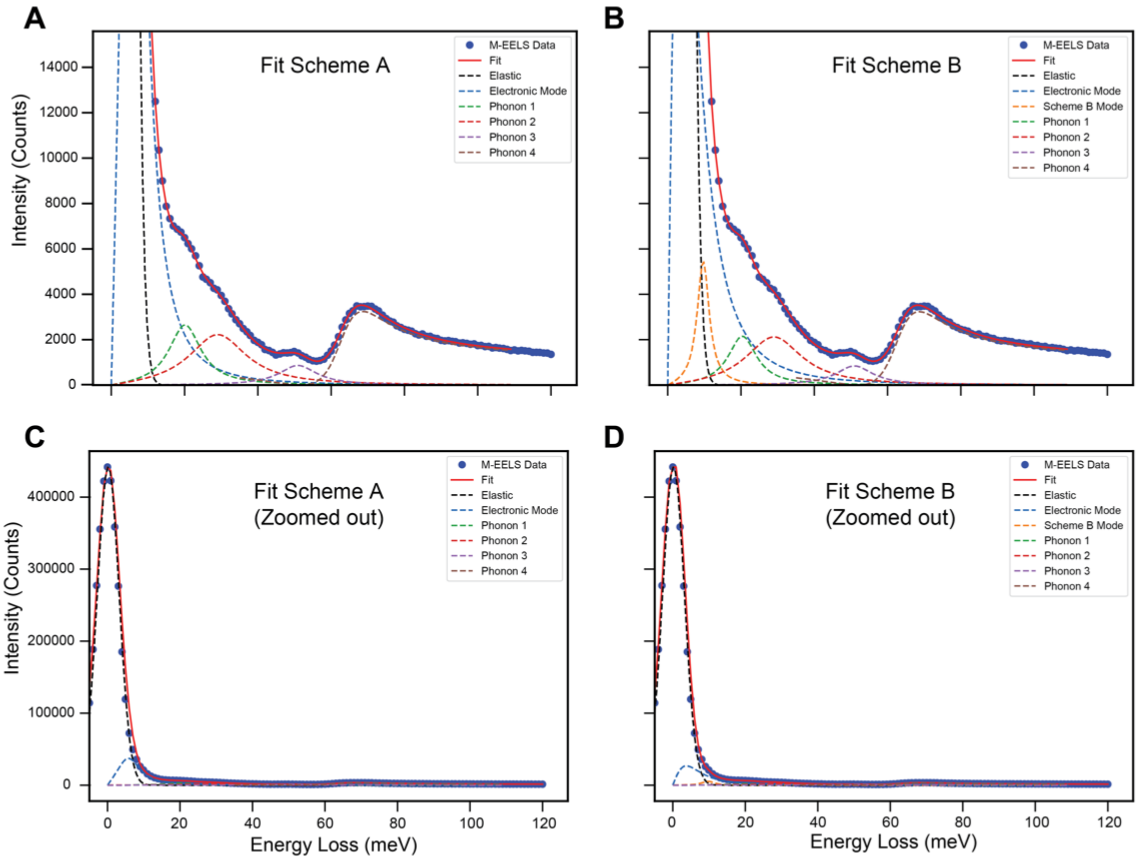


FIG. S9. **Fits estimates of the demon mode at small momentum**. Fits of the M-EELS spectra at $q = 0$ r.l.u. at $T = 300$ K where the demon mode is no longer clearly resolvable from the elastic line. To estimate an upper bound on its energy for $q < 0.02\text{Å}^{-1}$, the quasi-elastic line is fitted with a Gaussian, and the tails attributed to the demon mode in two schemes. In scheme A this tail is completely attributed to the demon, while in scheme B it is attributed to the sum of the demon and some other unresolvable mode with Lorentzian form. (A) Fit of the spectra according to scheme A as described in the text. (B) Fit of the same spectra as (A) but according to scheme B. (C) Same plot as (A) but vertical axis is zoomed out to show the quasi-elastic line and its tails. (D) Same plot as (B) but again zoomed out vertically.

## II. MULTI-BAND RPA CALCULATION

In order to understand the origin of the gapless made presented in the main manuscript, Fig. 3, we calculated the collective charge modes of $Sr_2RuO_4$ using Lindhard theory in the random phase approximation [17]. These calculations were performed without any adjustable parameters, without any optimization or fitting.

### A. Hamiltonian

We work with the following Hamiltonian as an effective description of the low-energy electronic degrees of freedom in $Sr_2RuO_4$ .

$$H = \sum_{k,s} \mathbf{c}_s^\dagger(k)\mathbf{A}_s(k)\mathbf{c}_s(k) + \frac{1}{2}\sum_q V(q)\rho(q)\rho(-q). \tag{1}$$

Here, $\mathbf{c}_s(k) = \left[d_s^{yz}(k)\ d_s^{xz}(k)\ d_{-s}^{xy}(k)\right]^T$ where $d_\sigma^i(k)$ annihilates an electron in orbital $i$ with spin $\sigma$ and momentum $k$. Following [18], we use a tight-binding band structure give by

$$\mathbf{A}_s(k) = \begin{bmatrix} \epsilon_k^{yz} - \tilde{\mu} & \epsilon_k^{\text{off}} + is\lambda & -s\lambda \\ \epsilon_k^{\text{off}} - is\lambda & \epsilon_k^{xz} - \tilde{\mu} & i\lambda \\ -s\lambda & -i\lambda & \epsilon_k^{xy} - \tilde{\mu} \end{bmatrix}, \tag{2}$$

where

$$\epsilon_k^{yz} = -2\tilde{t}_2\cos(k_x) - 2\tilde{t}_1\cos(k_y) \tag{3}$$

$$\epsilon_k^{xz} = -2\tilde{t}_1\cos(k_x) - 2\tilde{t}_2\cos(k_y) \tag{4}$$

$$\epsilon_k^{xy} = -2\tilde{t}_3(\cos(k_x) + \cos(k_y)) - 4\tilde{t}_4\cos(k_x)\cos(k_y) - 2\tilde{t}_5(\cos(2k_x) + \cos(2k_y)) \tag{5}$$

$$\epsilon_k^{\text{off}} = -4\tilde{t}_6\sin(k_x)\sin(k_y). \tag{6}$$

The parameters are determined in [18] by fitting to low energy photoemission spectra. In units of eV, the parameters are

| $\lambda$ | $\tilde{t}_1$ | $\tilde{t}_2$ | $\tilde{t}_3$ | $\tilde{t}_4$ | $\tilde{t}_5$ | $\tilde{t}_6$ | $\tilde{\mu}$ |
|---|---|---|---|---|---|---|---|
| 0.032 | 0.145 | 0.016 | 0.081 | 0.039 | 0.005 | 0.000 | 0.122 |

The Coulomb interaction is

$$V(q) = \frac{e^2}{\epsilon_0 \epsilon_\infty} \frac{1}{q^2} \tag{7}$$

$$= \left[ 0.313\,04\,\text{eV} \cdot \frac{\text{a}^2\text{c}}{2} \right] \frac{1}{\left[ q / \frac{2\pi}{\text{a}} \right]^2}. \tag{8}$$

We have used lattice constants a = 3.873 Å and c = 12.7323 Å from [19] and the high frequency dielectric constant $\epsilon_\infty = 2.3$ from [4]. $\frac{\text{a}^2\text{c}}{2}$ is the volume per Ru atom.

The charge density $\rho(q)$ is

$$\rho(q) = \sum_{k,s} \mathbf{c}_s^\dagger(k) \mathbf{c}_s(k+q). \tag{9}$$

We approximate the charge density of each orbital as entirely localized at the center of each Ru atom. This is a reasonable approximation at small $q$.

### B. Band basis

To facilitate calculations, we diagonalize the non-interacting part of the Hamiltonian

$$\mathbf{c}_s^\dagger(k) \mathbf{A}_s(k) \mathbf{c}_s(k) = \sum_{a,k} c_a^\dagger(k) \epsilon_a(k) c_a(k) \tag{10}$$

$$c_a(k) = \sum_i U_{ia}^*(k) c_i(k). \tag{11}$$

There are three bands, labeled $\alpha, \gamma, \beta$ in order of increasing energy. Each is doubly degenerate due to pseudospin. Therefore, in the following sections we work with one pseeudospin species and restore factors of 2 as necessary.

In the band basis, the charge density can be written as

$$\rho(q) = \sum_{iab,k} U_{ia}^*(k) U_{ib}(k+q) c_a^\dagger(k) c_b(k+q). \tag{12}$$

Therefore, the total density can be decomposed as

$$\rho(q) = \sum_{ab} \rho_{ab}(q) \tag{13}$$

$$\rho_{ab}(q) = \sum_{i,k} U_{ia}^*(k) U_{ib}(k+q) c_a^\dagger(k) c_b(k+q). \tag{14}$$

The density operator involves both band densities (e.g. $c_\alpha^\dagger c_\alpha$) and inter-band excitations (e.g. $c_\alpha^\dagger c_\beta$). This decomposition will be useful later in analyzing partial susceptibilties.

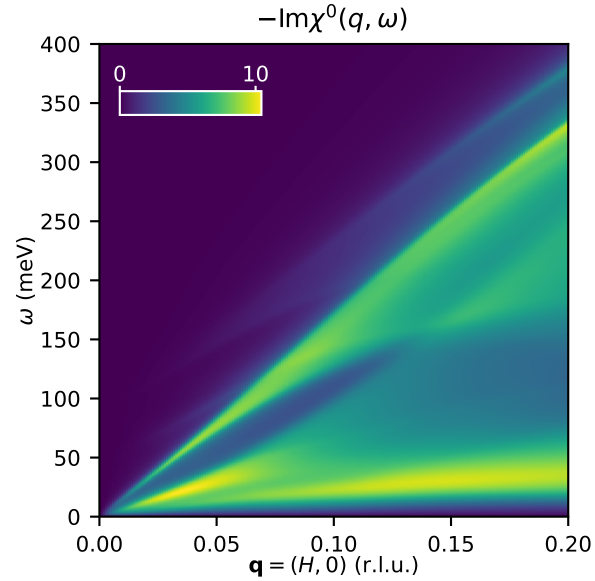


FIG. S10. **Noninteracting susceptibility of $\mathbf{Sr_2RuO_4}$ .** Negative of the imaginary part of $\chi^0(q,\omega)$ calculated using (15).

### C. Charge susceptibility

The non-interacting charge susceptibility is

$$\chi^0(q,\omega) = \frac{2}{N} \sum_{ijab,k} U_{ia}(k+q) U^*_{ja}(k+q) U_{jb}(k) U^*_{ib}(k) \frac{f(\epsilon_b(k)) - f(\epsilon_a(k+q))}{\omega + \epsilon_b(k) - \epsilon_a(k+q) + i0^+}. \tag{15}$$

Here, $i, j$ are orbital indices and $a, b$ are band indices. $N$ is the number of $k$-points summed over and $f(\epsilon) = \left(e^{\epsilon/T}+1\right)^{-1}$ is the Fermi-Dirac function. In figures showing the demon, we use a $1000 \times 1000$ grid of $k$-points uniformly distributed over the first Brillouin zone. The temperature is set to 30 K and a small Lorentzian broadening of $\gamma = 3\,\text{meV}$ is applied through substituting $i0^+ \to i\gamma$. In figures showing the plasmon, we use a $400 \times 400$ grid of $k$-points and a Lorentzian broadening of $\gamma = 10\,\text{meV}$. A plot of $-\operatorname{Im}\chi^0(q,\omega)$ is shown in Fig. S10. The features seen here may be understood through the band decomposition described in the next section.

Under the RPA, the full charge susceptibility is given by

$$\chi(q,\omega) = \frac{\chi^0(q,\omega)}{1 - V(q)\chi^0(q,\omega)}. \tag{16}$$

The result is plotted in Fig. 2a, 2b, and S11.

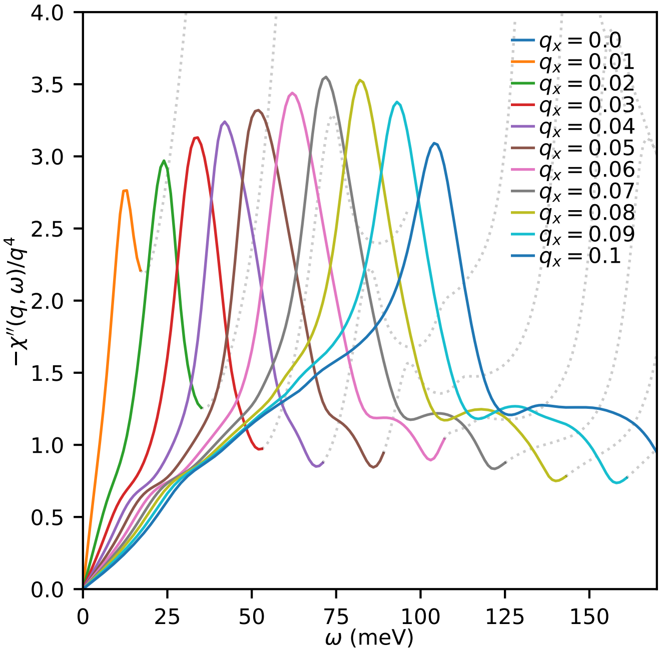


FIG. S11. **Imaginary part of the charge susceptibility at small momenta.** Divided by $q^4$ to highlight the demon.

### D. Demon intensity

The imaginary part of the total charge susceptibility calculated by RPA is plotted against frequency in Fig. S11 at small $q$. The linearly-dispersing demon is the most prominent feature at these momenta. Its peak intensity scales approximately as $q^4$. Given that the peak width also increases with $q$, the demon clearly fails to satisfy the $f$-sum rule, consistent with expectations for a neutral excitation (see main text and Section III below).

### E. Band decomposition of charge susceptibility

The susceptibility describes the response of the total charge density to a potential that couples to the total charge density. Since charge density can be decomposed into components in (13), we define a susceptibility matrix $\boldsymbol{\chi}(q,\omega)$ where each element describes the response of a component of the charge density to a potential that couples to a single component. To be precise,

$$\chi_{ab,cd}(q, i\omega_n) = -\frac{1}{N}\int_0^\beta \mathrm{d}\tau\, e^{i\omega_n\tau}(\langle\rho_{ab}(q,\tau)\rho_{cd}(-q)\rangle - \langle\rho_{ab}(q)\rangle\langle\rho_{cd}(-q)\rangle). \tag{17}$$

The susceptibility follows after analytically continuing $i\omega_n \to \omega + i0^+$. The non-interacting result is

$$\chi^0_{ab,cd}(q,\omega) = \delta_{ad}\delta_{bc}\frac{2}{N}\sum_{ij,k} U_{ia}(k+q)U^*_{ja}(k+q)U_{jb}(k)U^*_{ib}(k)\frac{f(\epsilon_b(k)) - f(\epsilon_a(k+q))}{\omega + \epsilon_b(k) - \epsilon_a(k+q) + i0^+}. \quad (18)$$

The delta functions are due to the decoupling of bands in a non-interacting system. For instance, if $a \neq d$, $\langle c^\dagger_a c_b c^\dagger_c c_d \rangle = \langle c^\dagger_a c_b \rangle \langle c^\dagger_c c_d \rangle$, so $\chi_{ab,cd} = 0$. In an interacting system, this is no longer true and all $9 \times 9$ elements of $\chi_{ab,cd}$ are nonzero in general.

The 9 nonzero elements of $\boldsymbol{\chi}^0(q,\omega)$ are plotted in Fig. S12. From this we can identify features in Fig. S10 as either intra-band or inter-band excitations. At small $q$, inter-band transitions have intensity $\sim q^2$ in $\chi^0(q,\omega)$ and therefore intra-band particle-hole excitations dominate. As can be seen in Fig. S12, the strongest contributors to $\chi^0$ are $\chi^0_{\gamma\gamma,\gamma\gamma}$ and $\chi^0_{\beta\beta,\beta\beta}$. The two bands clearly have different velocities. Importantly, at small $q$, $\mathrm{Im}\,\chi^0_{\beta\beta,\beta\beta}$ has spectral weight restricted to a small window of frequencies. This is due to the quasi-1d nature of the $\beta$ band. The consequence is that there is a pocket in $\mathrm{Im}\,\chi^0(q,\omega)$ from $q = (0,0)$ to $q \approx (0.13, 0)$ with suppressed spectral weight (Fig. S10). It is precisely in this pocket that the demon disperses (Fig. 2c) without becoming overdamped.

The interaction $V(q)\rho(q)\rho(-q)$ may be written as

$$V(q)\rho(q)\rho(-q) = \sum_{abcd} V_{ab,cd}(q)\rho_{ab}(q)\rho_{cd}(-q), \quad (19)$$

where $V_{ab,cd}(q) = V(q)$ for all $a, b, c, d$. Therefore, we define the $9 \times 9$ interaction matrix $\mathbf{V}(q)$ with every element equal to $V(q)$.

Under the RPA, the matrix susceptibility is

$$\boldsymbol{\chi}(q,\omega) = \boldsymbol{\chi}^0(q,\omega) + \boldsymbol{\chi}^0(q,\omega)\mathbf{V}(q)\boldsymbol{\chi}^0(q,\omega) + \cdots \quad (20)$$

$$= \boldsymbol{\chi}^0(q,\omega)\left[\mathbf{I} - \mathbf{V}(q)\boldsymbol{\chi}^0(q,\omega)\right]^{-1}, \quad (21)$$

where $\mathbf{I}$ is the identity matrix and multiplication and inversion are matrix operations. It is straightforward to show that the sum of all elements in the RPA susceptibility matrix equals the scalar RPA result in (16).

Density-density components of the susceptibility matrix ($\chi_{aa,bb}$) may be used to determine the identity of modes in $\chi(q,\omega)$. $\chi_{aa,bb}(q,\omega)$ describes the response of the density in band $a$ to a potential that couples to the density of band $b$. These components are plotted at high

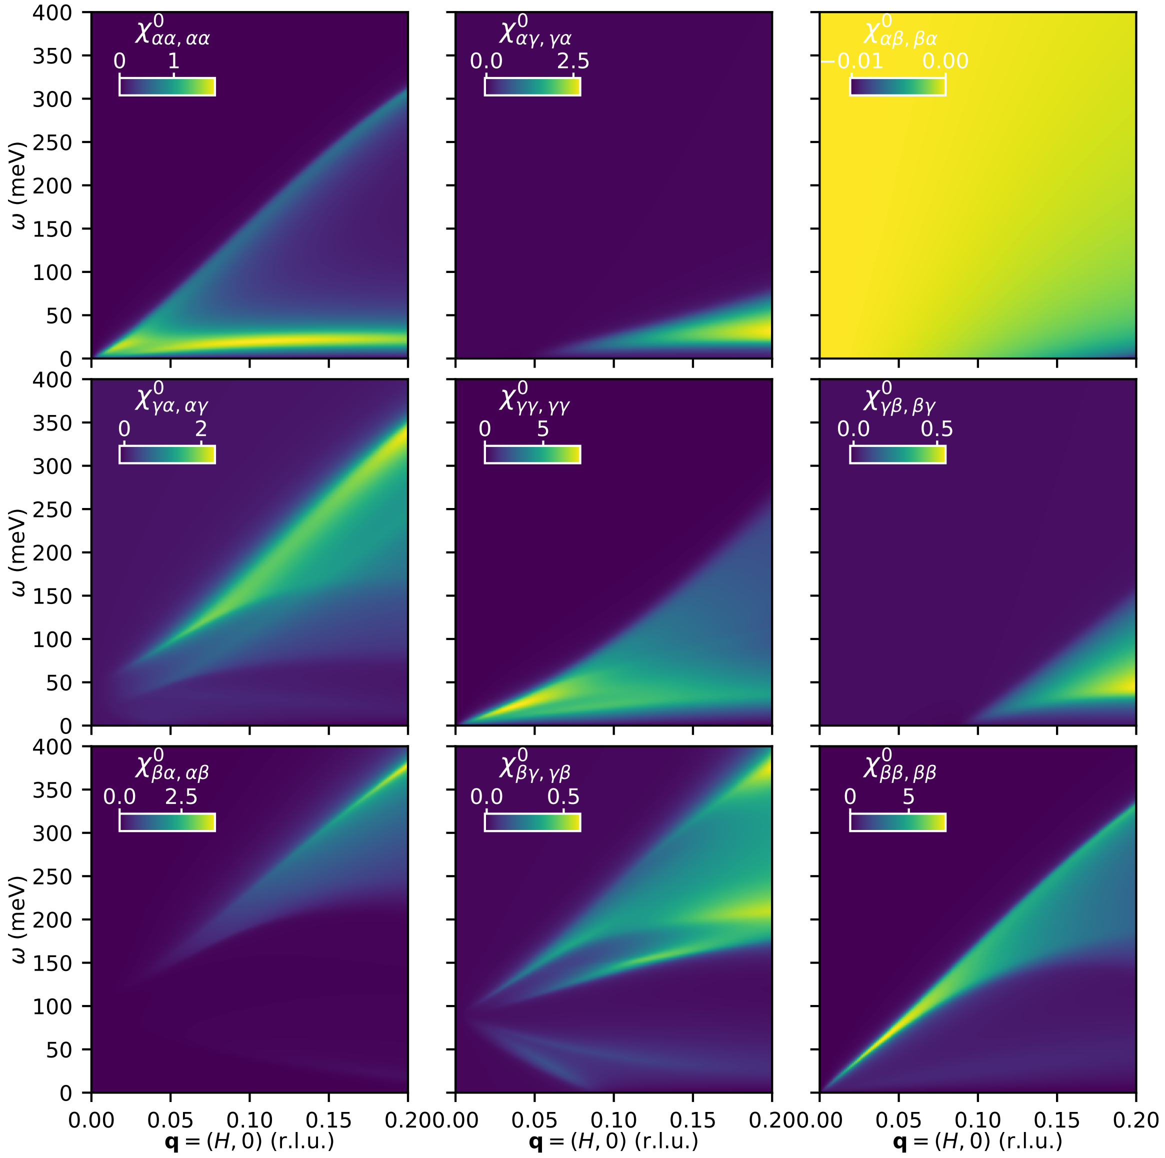


FIG. S12. **All nonzero elements of the non-interacting susceptibility matrix.** Diagonal elements show the particle-hole continua of the bands. Off-diagonal elements of the form $\chi_{ab,ba}$ show inter-band transitions from band $b$ to band $a$. Intensity corresponds to the negative of the imaginary part.

frequency in Fig. S13 and at low frequency in Fig. S14. Some of these components were plotted previously in Fig. 2, where we relabeled $\chi_{aa,bb} \equiv \chi_{a,b}$ for simplicity.

At high frequencies (Fig. S13), the plasmon is visible in all density-density components. Every component has the same sign, indicating that a potential modulated at the plasmon frequency induces an in-phase oscillation of the density in all three bands. By contrast, at low

frequencies (Fig. S14), a number of features are present including remnants of the particle-hole continua (Fig. S12) and the demon. The demon is visible most clearly in the elements $\chi_{\gamma\gamma,\gamma\gamma}$, $\chi_{\beta\beta,\beta\beta}$, $\chi_{\gamma\gamma,\beta\beta}$, and $\chi_{\beta\beta,\gamma\gamma}$. The sign of the susceptibility of the demon excitation in the diagonal elements, $\chi_{\gamma\gamma,\gamma\gamma}$ and $\chi_{\beta\beta,\beta\beta}$, is opposite to that of the off-diagonal elements, $\chi_{\gamma\gamma,\beta\beta}$, and $\chi_{\beta\beta,\gamma\gamma}$. This demonstrates the out-of-phase character of the demon. A potential coupling to the $\beta$ band that is modulated at the frequency of the demon excites opposite density modulations in the $\gamma$ and $\beta$ bands. This identifies the gapless mode in Fig. S14 as a true demon that, to leading order, does not modulate the total density.

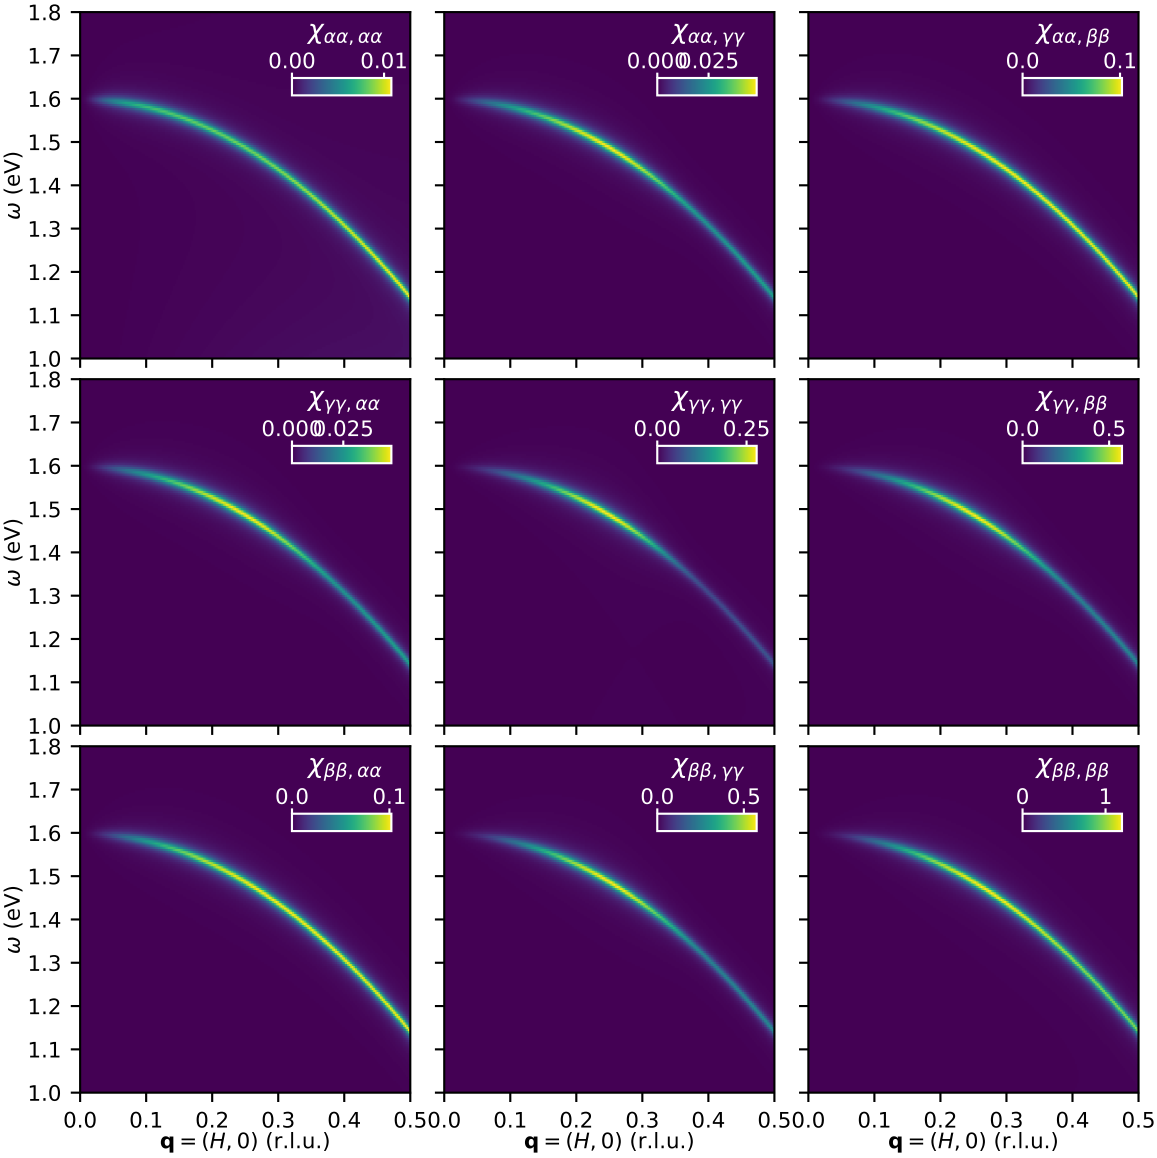


FIG. S13. **Density-density elements of the susceptibility matrix at high frequency.** Intensity corresponds to the negative of the imaginary part.

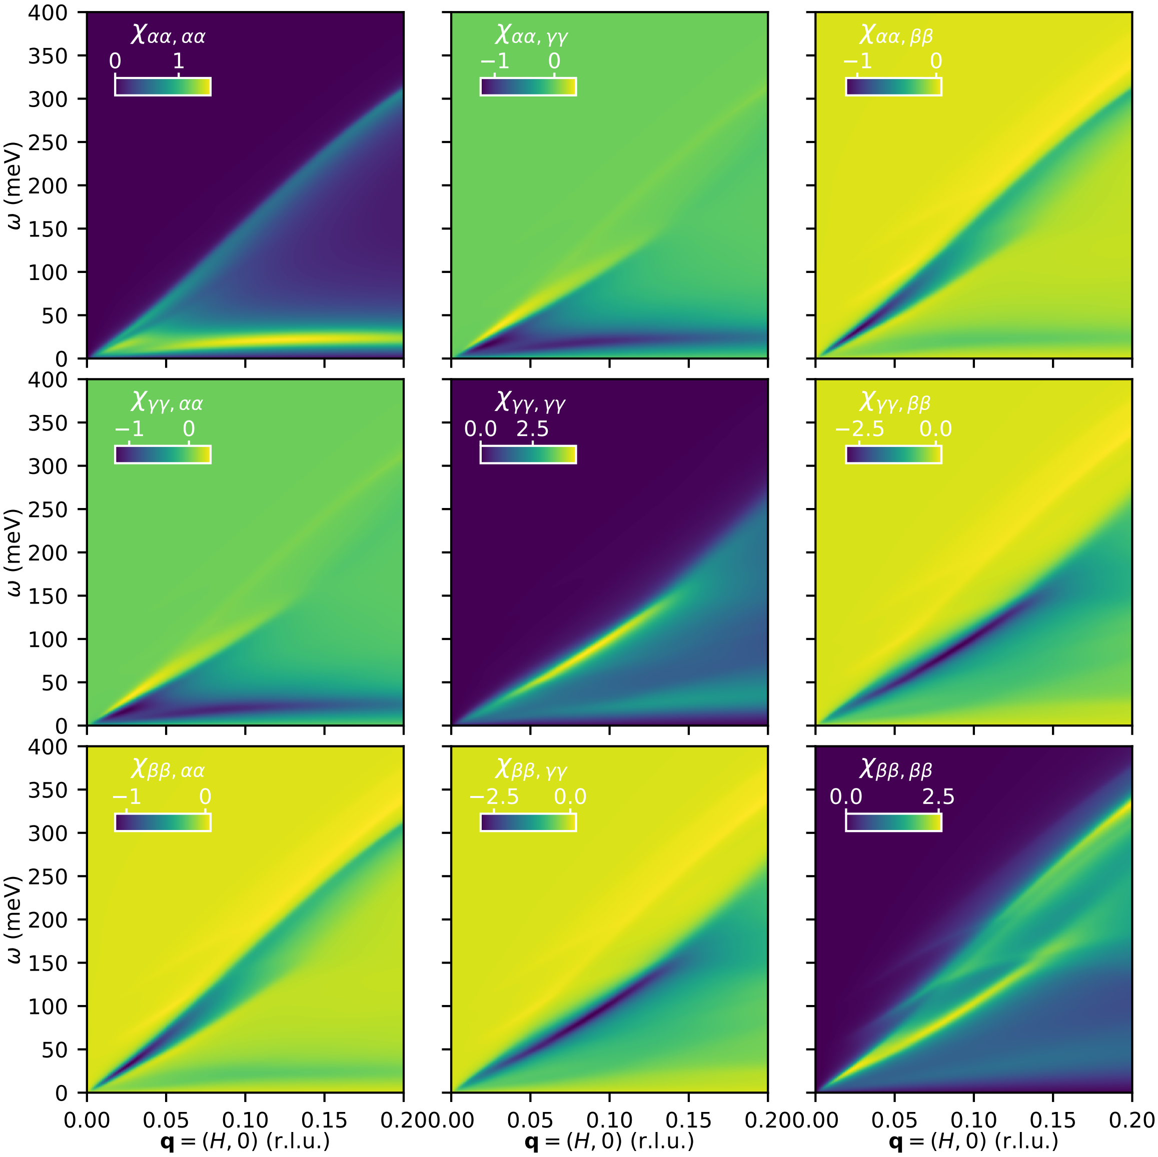


FIG. S14. **Density-density elements of the susceptibility matrix at low frequency.** Intensity corresponds to the negative of the imaginary part.

## III. SUM RULE FOR SURFACE EELS AND NEUTRALITY OF THE DEMON

A demon has two defining properties. The first is that it is gapless, i.e., its energy tends toward zero as $q \to 0$. The second is that it is neutral, i.e., it cannot screen charge in the $q \to 0$ limit. The former property is a consequence of the latter, which eliminates the Coulomb contribution to the energy of the mode in the long-wavelength limit. Fig. 4 of the main manuscript demonstrates that the collective mode is gapless. Here we show that it is also neutral, and therefore satisfies all the criteria for being a demon.

We can establish experimentally whether the excitation is neutral by examining the momentum dependence of its intensity. The dielectric function of a material is related to its charge susceptibility, $\chi(q, \omega)$, by

$$\epsilon(q, \omega) = \frac{1}{1 + V(q)\chi(q, \omega)} \tag{22}$$

where $V(q) = e^2/\epsilon_0 q^2$ is the 3D Coulomb interaction. The imaginary part of the susceptibility satisfies the $f$-sum rule,

$$\int_0^\infty \chi''(q, \omega)\, \omega\, d\omega = \frac{\pi n q^2}{2m}. \tag{23}$$

In conventional metals, the spectral weight in the plasmon takes up all the weight in this sum rule, and the intensity of the plasmon $\sim q^2$ at small $q$ (see, for example, Fig. 1 in Ref. [20]). This behavior assures that $V(q)\chi(q, \omega)|_{\omega=0}$ converges to a constant at small $q$, allowing the material to exhibit a finite screening strength.

In the RPA calculation described in Section II (summarized in Fig. 2 of the main manuscript), the spectral weight in the demon is a *faster* function of $q$ than the $f$-sum rule, i.e., $\chi \sim q^\alpha$, where $\alpha > 2$ ($\alpha = 4$ in the RPA case). Hence, for a demon excitation, $V(q)\chi(q, \omega)|_{\omega=0} \to 0$ as $q \to 0$, so $\epsilon \to 1$ and a demon does not contribute to screening in the long-wavelength limit. This is what is meant by the statement that a demon is "neutral." Determining whether the gapless mode in Fig. 4 of the main manuscript is neutral requires comparing the $q$-dependence of its spectral weight to expectations from the $f$-sum rule.

A complication is that M-EELS is a surface probe and does not measure the simple, bulk susceptibility, $\chi(q, \omega)$. M-EELS measures a surface response function, $\chi_s(q, \omega)$, as described in detail in Refs. [2, 21]. This surface quantity does not satisfy the same sum rule as Eq.

23, above. We therefore need to derive a sum rule for the response function measured with surface M-EELS, and compare the $q$-dependence of the spectral weight in the excitation to this sum rule.

### A. Sum rule for surface M-EELS

In general, the charge susceptibility can be written as

$$\chi(\mathbf{k},\mathbf{k}',\omega)=\sum_n\left\{\frac{\langle 0|\hat\rho_{\mathbf{k}}|n\rangle\langle n|\hat\rho_{-\mathbf{k}'}|0\rangle}{\omega-\omega_{n0}+i0_+}-\frac{\langle n|\hat\rho_{-\mathbf{k}'}|0\rangle\langle 0|\hat\rho_{\mathbf{k}}|n\rangle}{\omega+\omega_{n0}+i0_+}\right\}, \tag{24}$$

where $\hat\rho_{\mathbf{k}}$ is the charge density operator. In systems with translational symmetry, the only non-zero matrix elements of $\chi(\mathbf{k},\mathbf{k}',\omega)$ satisfy $\mathbf{k}=\mathbf{k}'+\mathbf{G}$, where $\mathbf{G}$ is a reciprocal lattice vector. In metals, where the system is completely homogeneous, $\mathbf{G}=0$. In systems that lack translational symmetry, the $f$-sum rule can be generalized to [17]

$$\int_{-\infty}^{\infty}\mathrm{d}\omega\,\omega\chi(\mathbf{k},\mathbf{k}',\omega)=i\pi\langle 0|[[\mathcal{H},\hat\rho_{-\mathbf{k}}],\hat\rho_{\mathbf{k}'}]|0\rangle. \tag{25}$$

The exact Hamiltonian $\mathcal{H}$ can be generically expressed in terms of the kinetic energy of free electrons, which is Galilean invariant, plus potentials that depend on charge density operators. In the absence of potentials that depend explicitly on momentum operators,

$$\langle 0|[[\mathcal{H},\hat\rho_{-\mathbf{k}}],\hat\rho_{\mathbf{k}'}]|0\rangle=-\frac{\hbar^2}{m}\mathbf{k}\cdot\mathbf{k}'\,\rho_{\mathbf{k}'-\mathbf{k}}. \tag{26}$$

The generalized $f$-sum rule then becomes

$$\int_{-\infty}^{\infty}\mathrm{d}\omega\,\omega\chi(\mathbf{k},\mathbf{k}',\omega)=-i\pi\frac{\hbar^2}{m}\mathbf{k}\cdot\mathbf{k}'\,\rho_{\mathbf{k}'-\mathbf{k}}. \tag{27}$$

We now wish to apply this sum rule to experimental M-EELS data. The M-EELS cross section is given by [2, 21]

$$\frac{\partial^2\sigma}{\partial\Omega\partial E}=\sigma_0V_{\mathrm{eff}}^2(\mathbf{q})\int_{-\infty}^{0}dz_1dz_2e^{-|\mathbf{q}||z_1+z_2|}\cdot S(\mathbf{q},z_1,z_2,\omega), \tag{28}$$

where $S$ is the density-density correlation function, which is related to the density response function by the fluctuation-dissipation theorem,

$$S(\mathbf{q},z_1,z_2,\omega)=-\frac{1}{\pi}\frac{1}{1-e^{-\hbar\omega/k_BT}}\chi''(\mathbf{q},z_1,z_2,\omega), \tag{29}$$

The Coulomb matrix elements

$$V_{\text{eff}}(k_z^i + k_z^s, q) = \frac{e^2/\epsilon_0}{(k_z^i + k_z^s)^2 + q^2} \tag{30}$$

describe the coupling of the probe electron to the valence electrons near a surface, accounting for a single reflectivity event [2, 21]

In a semi-infinite stack of metallic layers, translational symmetry is satisfied along the directions parallel to the metallic layers, but not in the direction perpendicular to the surface. The susceptibility has the general form $\chi(\mathbf{q}, \mathbf{q}, k_z, k_z')$, with $\mathbf{q}$ the momentum parallel to the surface and $k_z$, $k_z'$ the momenta along the direction perpendicular to the surface. Fourier transforming (27) in $k_z$ and $k_z'$, the generalized $F$-sum rule can be equivalently written as

$$\int_{-\infty}^{\infty} \mathrm{d}\omega\omega\, \chi(\mathbf{q}, \mathbf{q}, z, z', \omega) = -i\pi\frac{\hbar^2}{m}\left[\delta(z-z')q^2 - \frac{\partial^2\delta(z-z')}{\partial(z-z')^2} + \frac{\partial\delta(z-z')}{\partial(z-z')}\frac{\partial}{\partial z'}\right]\rho(z'), \tag{31}$$

where because of the surface $\rho(z) = 0$ for $z > 0$. Combining the scattering cross section of M-EELS [2, 21],

$$\frac{\partial^2\sigma}{\partial\Omega\partial E}(\mathbf{q}, k_z^i, k_z^s, \omega) = -\frac{1}{\pi}\frac{1}{1-\mathrm{e}^{-\beta\omega}}\sigma_0\left[V_{\text{eff}}(k_z^i + k_z^s, \mathbf{q})\right]^2 \int_{-\infty}^{0} \mathrm{d}z_1\mathrm{d}z_2\mathrm{e}^{q(z_1+z_2)}\mathrm{Im}\chi(\mathbf{q}, \mathbf{q}, z_1, z_2, \omega), \tag{32}$$

with the $f$-sum rule (31), the sum rule for the M-EELS cross section is

$$\int_{-\infty}^{\infty} \mathrm{d}\omega\, \omega(1-\mathrm{e}^{-\beta\omega})\frac{\partial^2\sigma}{\partial\Omega\partial E}(\mathbf{q}, k_z^i, k_z^s, \omega) = \frac{2\hbar^2q^2}{m}\sigma_0\left[V_{\text{eff}}(k_z^i + k_z^s, \mathbf{q})\right]^2 \int_{-\infty}^{0} \mathrm{d}z\rho(z)\mathrm{e}^{2qz}. \tag{33}$$

### B. Neutrality test of the collective mode

Eq. 33 is written in terms of the experimental cross section and therefore may be applied directly to the experimental data. We start by making some simplifying assumptions that apply in the small $q$ regime. The first is that the density $\rho(z) = \rho_0\,\theta(-z)$, i.e.,

$$\int_{-\infty}^{0} dz\,\rho(z)\,e^{2qz} = \frac{\rho_0}{2q} \tag{34}$$

This expression is valid as long as the width of the surface (i.e., the distance over which the density falls to zero) is much less than $q^{-1}$. Next, we take $T = 0$, which for data taken at $T = 30$ K is valid for $\omega > 2.5$ meV. Finally, we need to consider the actual behavior of the

mode in the small $q$ regime. While the mode disperses linearly over most of its range, in the small $q$ limit $E(q) \sim q^2$. We therefore take the experimental intensity to have the form

$$I(q, \omega) = I_0(q)\, \delta(\omega - \alpha q^2) \tag{35}$$

where $I_0(q)$ then represents the $\omega$-integrated intensity of the mode at momentum $q$. Evaluating Eq. 33 then gives

$$I_0(q) = \frac{\hbar^2 \sigma_0 e^2 \rho_0}{m \epsilon_0 \alpha} \frac{1}{q^5}. \tag{36}$$

In other words, if a collective mode encompasses all the spectral weight in the $f$-sum rule, its integrated intensity should satisfy Eq. 36. If, however, a mode is neutral, its spectral weight should scale with a higher power of $q$. In other words, for a given excitation, $I_0(q) \sim q^{\phi}$ in the small $q$ limit. If the excitation is neutral, then $\phi > -5$.

We carried out this test on the gapless excitation observed with M-EELS in Fig. 4. The result is shown in Fig. 4(d). The integrated intensity of the mode follows a power law of roughly $I_0(q) \sim q^{-1.8}$. Because -1.8 > -5, we conclude that this excitation is neutral in the sense that it cannot contribute to screening in the small $q$ limit, and therefore is a demon in the true sense.

---


[1] R. Fittipaldi, A. Vecchione, S. Fusanobori, K. Takizawa, H. Yaguchi, J. Hooper, R. Perry, and Y. Maeno, Journal of Crystal Growth **282**, 152 (2005).

[2] S. Vig, A. Kogar, M. Mitrano, A. A. Husain, V. Mishra, M. S. Rak, L. Venema, P. D. Johnson, G. D. Gu, E. Fradkin, M. R. Norman, and P. Abbamonte, SciPost Physics **3**, 026 (2017).

[3] J. Li, Z. Lin, G. Miao, W. Zhong, S. Xue, Y. Li, Z. Tao, W. Wang, J. Guo, and X. Zhu, Surface Science **721**, 122067 (2022).

[4] D. Stricker, J. Mravlje, C. Berthod, R. Fittipaldi, A. Vecchione, A. Georges, and D. van der Marel, Physical Review Letters **113**, 087404 (2014).

[5] A. A. Husain, M. Mitrano, M. S. Rak, S. Rubeck, B. Uchoa, K. March, C. Dwyer, J. Schneeloch, R. Zhong, G. D. Gu, and P. Abbamonte, Physical Review X **9**, 041062 (2019).

[6] M. Mitrano, A. A. Husain, S. Vig, A. Kogar, M. S. Rak, S. I. Rubeck, J. Schmalian, B. Uchoa,

J. Schneeloch, R. Zhong, G. D. Gu, and P. Abbamonte, Proceedings of the National Academy of Sciences **115**, 5392 (2018), https://www.pnas.org/doi/pdf/10.1073/pnas.1721495115.

[7] B. Stöger, M. Hieckel, F. Mittendorfer, Z. Wang, D. Fobes, J. Peng, Z. Mao, M. Schmid, J. Redinger, and U. Diebold, Physical Review Letters **113**, 116101 (2014).

[8] A. Tamai, M. Zingl, E. Rozbicki, E. Cappelli, S. Riccò, A. de la Torre, S. McKeown Walker, F. Y. Bruno, P. D. C. King, W. Meevasana, M. Shi, M. Radović, N. C. Plumb, A. S. Gibbs, A. P. Mackenzie, C. Berthod, H. U. R. Strand, M. Kim, A. Georges, and F. Baumberger, Physical Review X **9**, 021048 (2019).

[9] K. M. Shen, A. Damascelli, D. H. Lu, N. P. Armitage, F. Ronning, D. L. Feng, C. Kim, Z.-X. Shen, D. J. Singh, I. I. Mazin, S. Nakatsuji, Z. Q. Mao, Y. Maeno, T. Kimura, and Y. Tokura, Physical Review B **64**, 180502 (2001).

[10] A. Damascelli, K. Shen, D. Lu, N. Armitage, F. Ronning, D. Feng, C. Kim, Z.-X. Shen, T. Kimura, Y. Tokura, Z. Mao, and Y. Maeno, Journal of Electron Spectroscopy and Related Phenomena **114-116**, 641 (2001), proceeding of the Eight International Conference on Electronic Spectroscopy and Structure,.

[11] B. Diaconescu, K. Pohl, L. Vattuone, L. Savio, P. Hofmann, V. M. Silkin, J. M. Pitarke, E. V. Chulkov, P. M. Echenique, D. Farías, and M. Rocca, Nature **448**, 57 (2007).

[12] S. J. Park and R. E. Palmer, Physical Review Letters **105**, 016801 (2010).

[13] Ismail, J. Zhang, R. Matzdorf, T. Kimura, Y. Tokura, and E. W. Plummer, Physical Review B **67**, 10.1103/physrevb.67.035407 (2003).

[14] A. P. Mackenzie and Y. Maeno, Reviews of Modern Physics **75**, 657 (2003).

[15] Z. Wang, D. Walkup, P. Derry, T. Scaffidi, M. Rak, S. Vig, A. Kogar, I. Zeljkovic, A. Husain, L. H. Santos, Y. Wang, A. Damascelli, Y. Maeno, P. Abbamonte, E. Fradkin, and V. Madhavan, Nature Physics **13**, 799 (2017).

[16] M. Braden, W. Reichardt, Y. Sidis, Z. Mao, and Y. Maeno, Physical Review B **76**, 014505 (2007).

[17] D. Pines and P. Nozières, *The Theory of Quantum Liquids* (Perseus Books, Cambridge, MA, 1999).

[18] V. Zabolotnyy, D. Evtushinsky, A. Kordyuk, T. Kim, E. Carleschi, B. Doyle, R. Fittipaldi, M. Cuoco, A. Vecchione, and S. Borisenko, Journal of Electron Spectroscopy and Related

Phenomena **191**, 48 (2013).

[19] Q. Huang, J. Soubeyroux, O. Chmaissem, I. Sora, A. Santoro, R. Cava, J. Krajewski, and W. Peck, Journal of Solid State Chemistry **112**, 355 (1994).

[20] P. Abbamonte, K. D. Finkelstein, M. D. Collins, and S. M. Gruner, Phys. Rev. Lett. **92**, 237401 (2004).

[21] E. Evans and D. L. Mills, Phys. Rev. B **5**, 4126 (1972).
